# Supplementary material for: Additive rule of real and reciprocal space topologies at disclinations
Source: arXiv:2202.09560 source file (2022-02-19)
Supplement: Supplementary file 1 [file Supplementary.pdf]

# Supplemental Information for
# "Additive rule of real and reciprocal topologies at disclinations"

Qinghua He, Jinhua Sun, Hai-Yao Deng, Katsunori Wakabayashi and Feng Liu

## A. The vectored topological invariant for a disclination

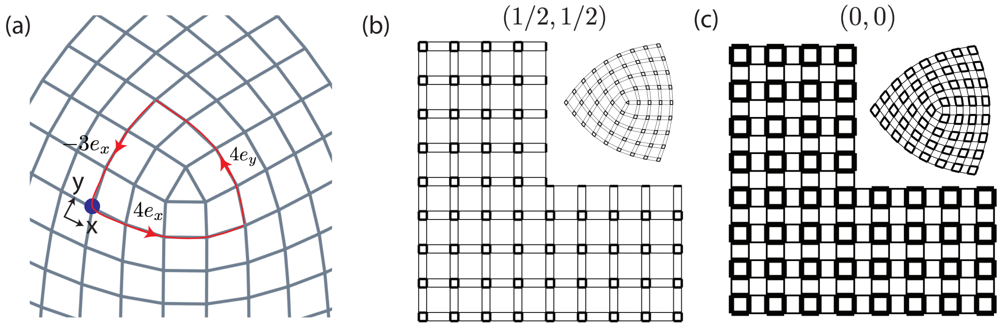


Figure S1: (a): Schematic of a disclination with $\Omega = -\frac{\pi}{2}$. For the loop shown here, $\mathbf{B} = e_x + 4e_y$. (b) and (c): Disclination types in the 2D SSH model for $\Omega = -\frac{\pi}{2}$, with $\mathbf{s} = (\frac{1}{2}, \frac{1}{2})$ and $\mathbf{s} = (0, 0)$, respectively. $\mathbf{s}$ indicates the rotational center of the sample.

Here we discuss the topological invariant of disclinations. As well known, a disclination is characterized by its Frank angle $\Omega$ and Burgers vector $\mathbf{B}$. For given $\Omega$, $\mathbf{B}$ can be evaluated by a holonomy along a closed path surrounding the disclination center. An example of $\mathbf{B}$ is displayed in Fig. S1 (a). Note that $\mathbf{B}$ depends on the starting (ending) point of the path and is hence not unique to the disclination. Nevertheless, it is easy to see that the parity of $2\mathbf{B}$, which we denote by $2\mathbf{s}$, is independent of the path and indeed unique. It univocally indicates the center of the wedge used in the Volterra construction of a disclination. For a sample possessing full point-group symmetry prior to Volterra process, $\mathbf{s}$ locates the rotational center of the sample and $2\mathbf{s}$ can be obtained by counting the number of unit cells (mod 2) along each axis. One may see that, for $\Omega = \pm\frac{\pi}{2}$, $\mathbf{s} \in \{(0, 0), (1/2, 1/2)\}$. For $\Omega = \pm\pi$, however, $\mathbf{s} \in \{(0, 0), (0, 1/2), (1/2, 0), (1/2, 1/2)\}$. Examples are shown in Figure S1 (b) and (c). This observation can also be reached by group-theoretic analysis. Note that $\mathbf{B}$ and $R_\theta\mathbf{B} - R_\Omega\mathbf{a} + \mathbf{a}$ represent different loops but enclosing the same disclination and should then be deemed equivalent. Here $(\theta, \mathbf{a})$ parameterizes a displacement by $\mathbf{a}$ and rotation by $\theta$ (denoted by $R_\theta$). The equivalence classes of $\mathbf{B}$ can be shown to form a $Z_2$ group for $\Omega = \pm\pi/2$ and a $Z_2 \otimes Z_2$ group for $\Omega = \pm\pi$.

## B. Reciprocal topology of the 2D SSH model

The Hamiltonian for the bulk 2D SSH model is given as

$$H(k_x, k_y) = \begin{pmatrix} 0 & \rho(k_x) & \rho(k_y) & 0 \\ \rho^*(k_x) & 0 & 0 & \rho(k_y) \\ \rho^*(k_y) & 0 & 0 & \rho(k_x) \\ 0 & \rho^*(k_y) & \rho^*(k_x) & 0 \end{pmatrix}, \tag{S1}$$

where $\rho(k) = \gamma + \gamma' e^{ika}$. The spectrum of $H$ is given by $E = s_1|\rho(k_x)| + s_2|\rho(k_y)|$ with $s_{1,2} = \pm 1$. The $C_4$ point-group symmetry dictates that there are two topologically distinct band structures depending on the ratio $\gamma/\gamma'$, see the left panel of Figure S2 (a). As displayed in the right panel of Figure S2 (a), a band inversion takes place at $\gamma = \gamma'$. The reciprocal-space topology of the model is determined by the parities of the lowest band at $\Gamma$ and $X(Y)$ points in the 1BZ, respectively. The nontrivial topological phase has opposite parities at $\Gamma$ and $X(Y)$ points for which the vectored Zak's phase equals to $(\pi, \pi)$.

In Fig. S2 (b) we display the charge distribution for a sample at 1/4 filling, where only the lowest energy band is occupied. As expected, 1/4 and 1/2 fractional charges appear in the nontrivial phase at corners and along edges, respectively.

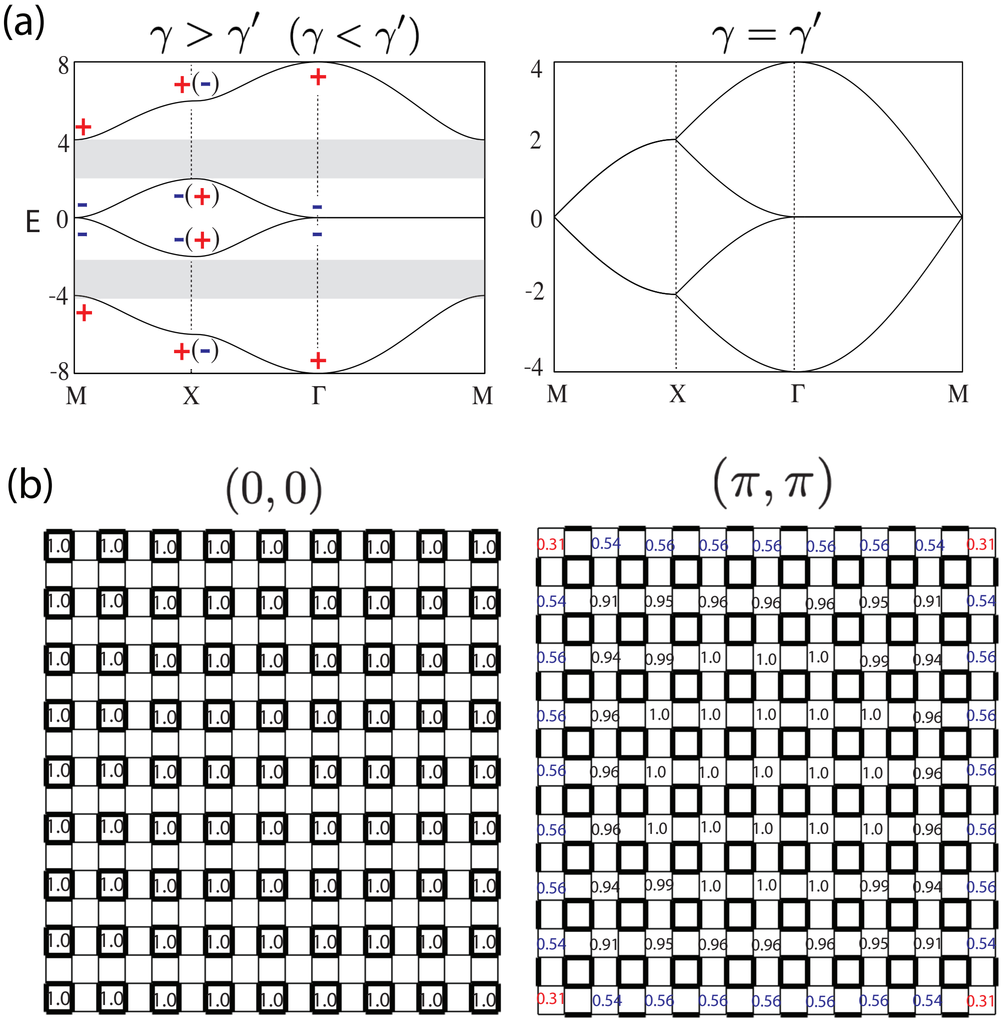


Figure S2: (a) Band structure of the 2D SSH model for $\gamma, \gamma' = 1.0, 3.0 (\gamma, \gamma' = 3.0, 1.0)$ and $\gamma = \gamma' = 1.0$. The signs ($\pm$) represent the parities of the wave function at the corresponding points in the 1BZ. Band inversion occurs at the X (Y) point. (b) Charge distribution in a sample: The left panel has vectored Zak's phase $(0, 0)$ while the right panel has $(\pi, \pi)$. The 1/4 corner fractional charge and 1/2 edge fractional charge are marked in red and blue, respectively.

## C. Half-bound states

To clarify that the half-bound state associated with the disclination with $\Omega = -\pi$ and $\mathbf{s} = (1/2, 0)$ is an instrinc state that is oblivious to sample size, we calculate it for a much larger sample as shown in Figure S3 (a). The nine eigenstates that are most concentrated about the disclination center are exhibited in panel (b). Clearly, the half-bound state forms here, just as in smaller samples shown in the main text.

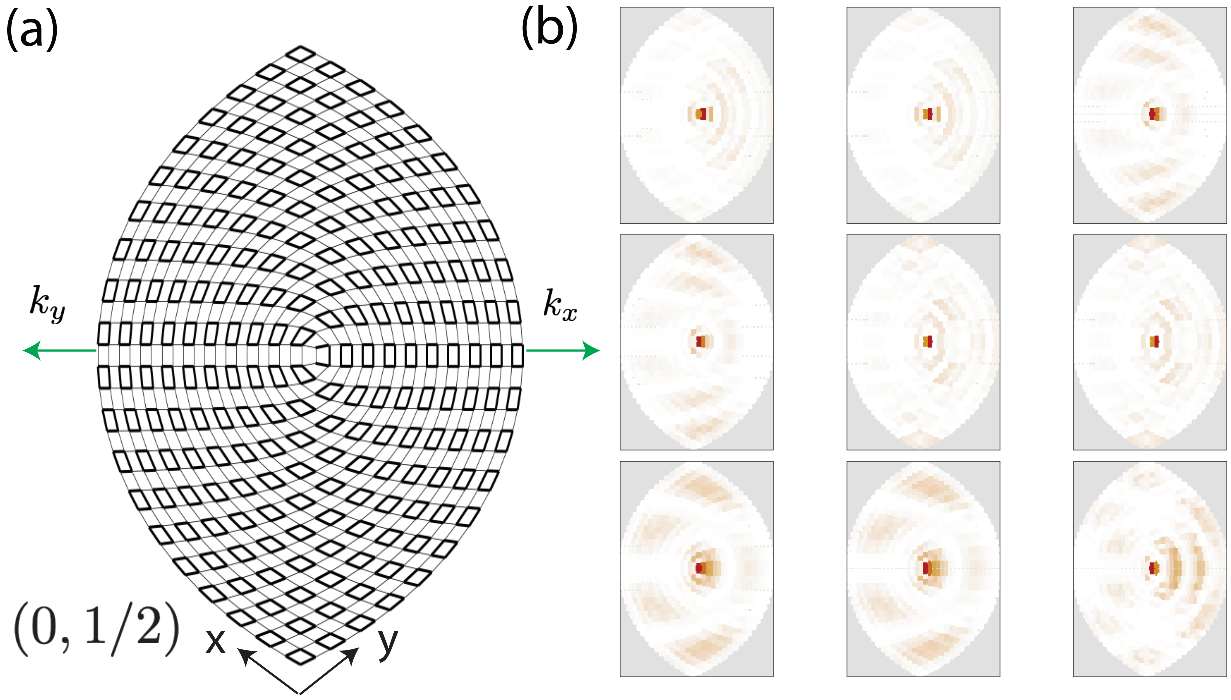


Figure S3: (a) Disclination with $\Omega = -\pi$ and $\mathbf{s} = (1/2, 0)$. (b) The nine eigenstates that are most concentrated about the disclination. $\mathbf{p} = (0, 0)$.

## D. Parameter pumping of ultra-stable bound states

It is worth discussing an adiabatic pumping as a means for exploiting the transition from real-space protected bound states to reciprocal-space protected ones at the disclination. To this end, we set $(\gamma, \gamma') = (3\cos\theta, 1)$ with $\theta$ being the pumping parameter. As $\mathbf{p}$ only depends on the ratio $|\gamma/\gamma'|$, we let $\theta$ vary from $-\pi/2$ to $\pi/2$. The pumping spectrum is plotted in Fig. S4. The bound states at the disclination show up as in-gap states. Compared with quantum pumping using topological edge states, the parameter pumping here causes spectral flow between bound states protected by real-space topology and those by reciprocal-space topology. As a result, the number of topological transport channels is not limited by the dimensions of systems such as edges and corners.

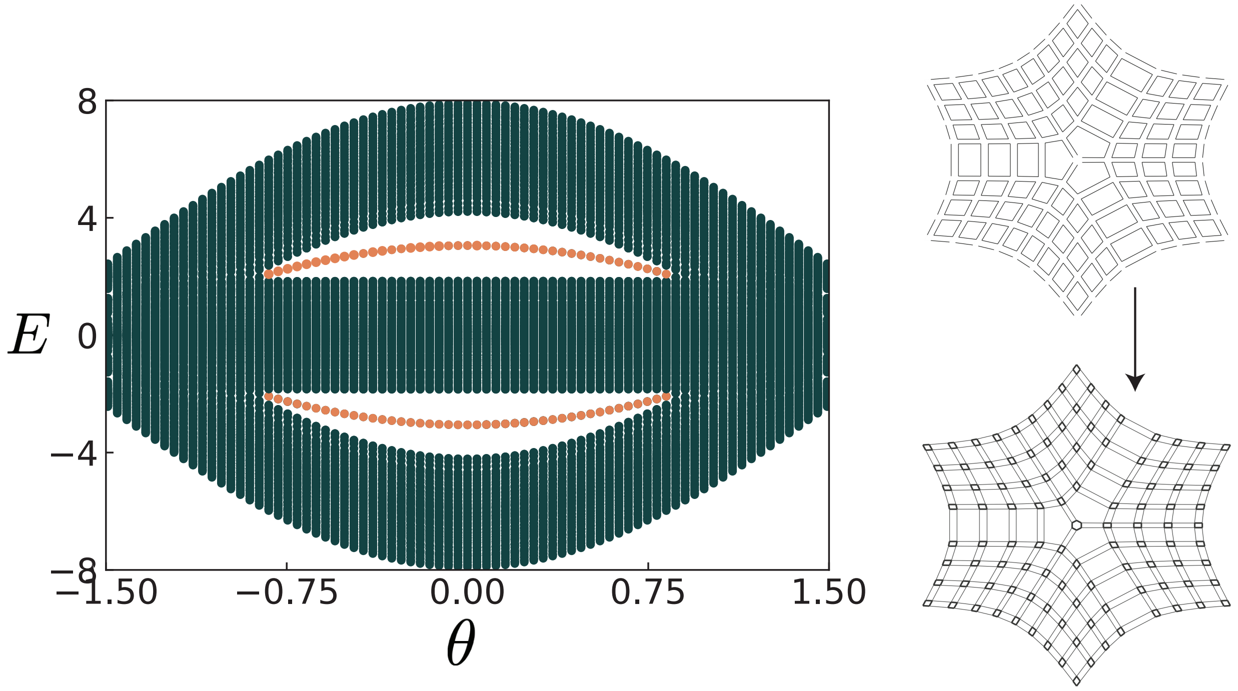


Figure S4: Topological parameter pumping by the disclination with $\Omega = \pi$ and $\mathbf{s} = (0, 1/2)$. The green is the energy spectra of the bulk and edge states, and orange is that of the bound states at the disclination. Bound states (including corner states) buried in the spectra of edge and bulk states are not shown.
